# Supplementary material for: Broad diversity of near-infrared single-photon emitters in silicon
Source: arXiv:2010.11068 ancillary file (2020-10-23)
Supplement: Supplementary file 1 [file Durand_et_al_arXiv_Silicon_SM.pdf]

# Broad diversity of near-infrared single-photon emitters in silicon
# Supplemental Material

A. Durand,[1] Y. Baron,[1] W. Redjem,[1] T. Herzig,[2] A. Benali,[3] S. Pezzagna,[2] J. Meijer,[2] A. Yu. Kuznetsov,[4] J.-M. Gérard,[5] I. Robert-Philip,[1] M. Abbarchi,[3] V. Jacques,[1] G. Cassabois,[1] and A. Dréau[1,*]

[1]*Laboratoire Charles Coulomb, Université de Montpellier and CNRS, 34095 Montpellier, France*
[2]*Division of Applied Quantum Systems, Felix-Bloch Institute for Solid-State Physics, University Leipzig, Linnéestraße 5, 04103 Leipzig, Germany*
[3]*CNRS, Aix-Marseille Université, Centrale Marseille, IM2NP, UMR 7334, Campus de St. Jérôme, 13397 Marseille, France*
[4]*Department of Physics, University of Oslo, NO-0316 Oslo, Norway*
[5]*Department of Physics, IRIG-PHELIQS, Univ. Grenoble Alpes and CEA, F-38000 Grenoble, France*

## ADDITIONAL $g^{(2)}$ MEASUREMENTS

Figure S-1 show the second-order autocorrelation functions $g^{(2)}(\tau)$ measured on the emitters corresponding to the PL spectra presented on Fig. 1(c) of the main text. All curves present a clear antibunching effect at zero delay with $g^{(2)}(0) < 0.5$, evidencing the presence of individual defects emitting photons one by one. Three defects, SD-5, SD-6 and G-center, exhibit also a bunching effect associated with $g^{(2)}(\tau) > 1$. This behaviour indicates that the optical cycles include a non-radiative transition through a metastable state [1].

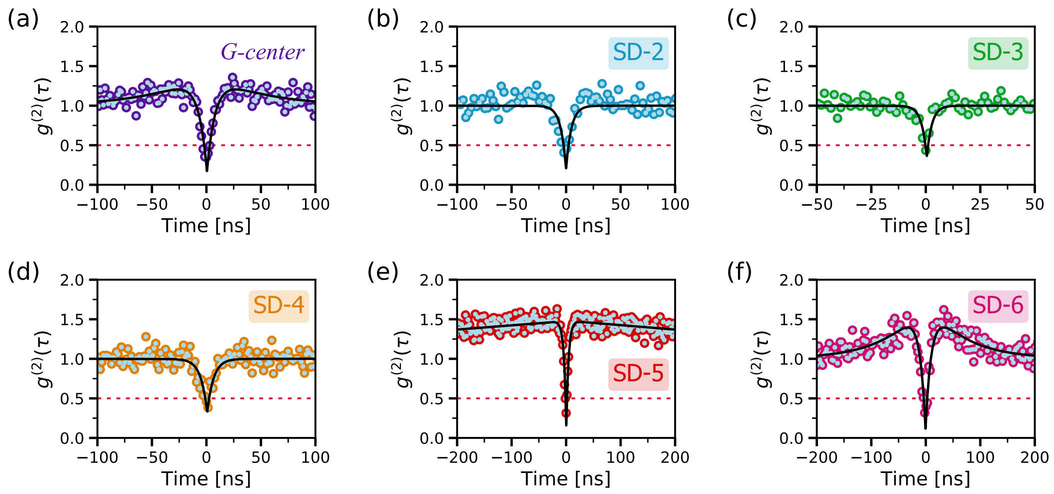


Figure. S-1. (a-f) Second-order autocorrelation function $g^{(2)}(\tau)$ corresponding to the single G-center and the individual defects from families SD-2 to SD-6 whose PL spectrum are presented on Fig. 1(c) of the main text. No background correction is applied and data are fitted with a two-level model (SD-2 to SD-4) or three-level model (G, SD4, SD-5) [1]. The optical power used is above the saturation power for each defect.

## EMISSION DIPOLE AND LIFETIME MEASUREMENTS FOR SD-5 AND SD-6

Figure S-2 display the complementary data from Figure 3 of the main text for individual defects from families SD-5 and SD-6. The emission polarization diagrams (Fig. S-2(a)) show a single emission dipole oriented respectively along the [110] and $[1\bar{1}0]$ crystal axis for these specific SD-5 and SD-6 emitters. Time-resolved PL measurements under pulsed laser excitation reveal a relaxation dynamics with two characteristic decay times: a short lifetime around 5 ns and a long one about 19 ns and 35 ns for SD-5 and SD-6 defects, respectively.

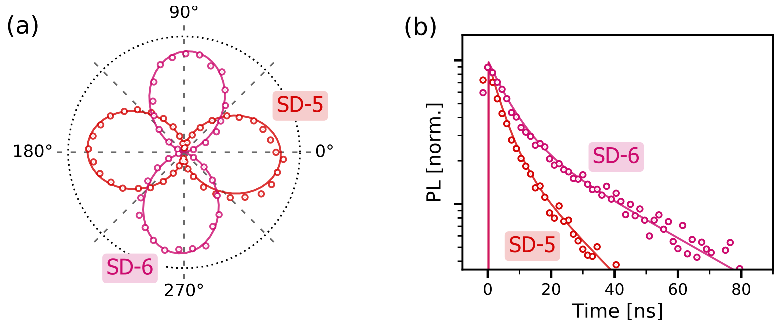


Figure. S-2. (a) Emission polarization diagram and (b) time-resolved PL decay measured on single SD-5 and SD-6 defects following the same procedure as indicated in the main text.

## VANISHING AND APPEARANCE OF SD-5 DEFECTS WITH THERMAL CYCLES

All defects discussed in this work are robust against repeated thermal cycles from 10 K to room-temperature, except SD-5 centers. We observed that thermal cycles of the cryostat can either destroy or create SD-5 emitters. Figure S-3(a) displays a first PL raster image measured at 10K that presents an isolated bright spot associated with a PL spectrum typical from SD-5 family (Fig. 3 (b)). After a cryostat warming-up to 300K, a second PL scan recorded at 10K on the same area shows that this emitter is no longer there (Fig. 3 (c)). On the contrary on other sample areas, we observe that the temperature increase can produce new fluorescing spots associated with SD-5 PL spectrum (Fig. 3 (d-f)).

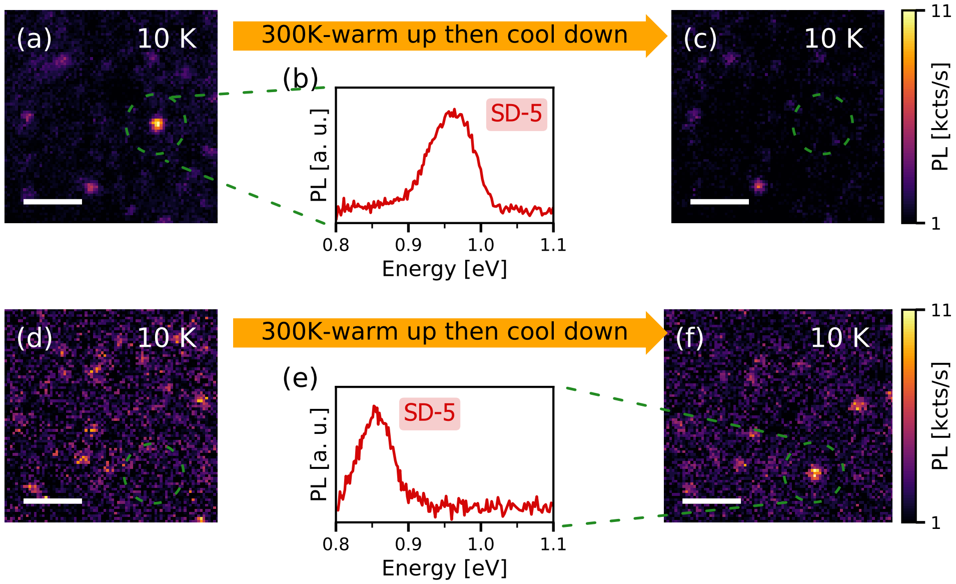


Figure. S-3. PL scans acquired at 10K on 2 sample areas (a,d) before and (c,f) after a warming-up of the cryostat to 300K. Horizontal bar corresponds to 5 μm. (b,e) PL spectra associated with SD-5 family and recorded on the bright spots circled on (a) and (f) respectively.

## EMISSION DIPOLE STABILITY WITH TEMPERATURE

To investigate potential atomic displacement that could impact their emission dipole [2, 3], we measured the emission polarization diagram of a single G-center and a single SD-2 defect at different temperatures (Fig. 4). No modification of the emission dipole has been observed while increasing the temperature up to 130 K for the G-center (Fig. 4 (a-c)) and up to 70K for the SD-2 emitter (Fig. 4 (d-f)).

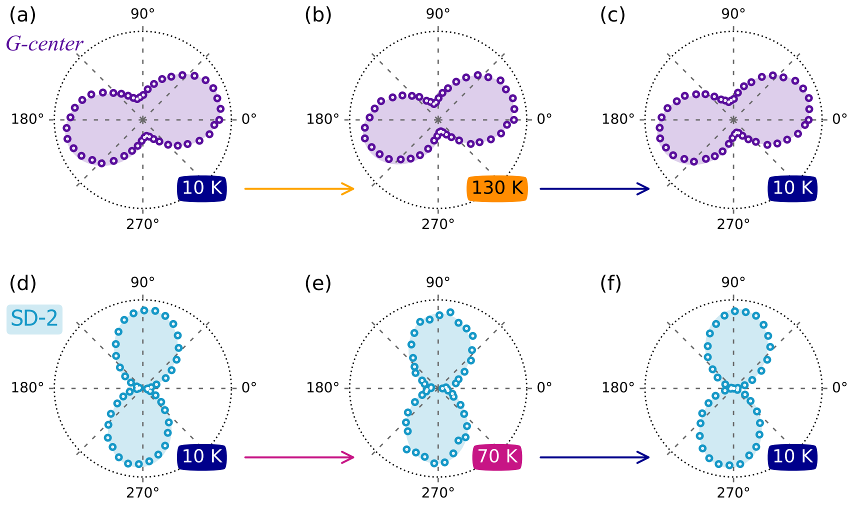


Figure. S-4. Emission diagram measured at different temperatures for (a-c) a single G-center and (d-e) a single SD-2 center. The lower PL contrast observed on the G-center data is due to imperfect background correction.

## EXCITED STATE LIFETIME EVOLUTION WITH TEMPERATURE

The excited-state lifetime measurements performed on a single G-center and a single SD-2 defect show that the higher the temperature, the shorter the PL decay (Fig. 5). The shortening of the defect lifetimes while increasing temperature is a common behaviour due to thermal activation of non-radiative processes.

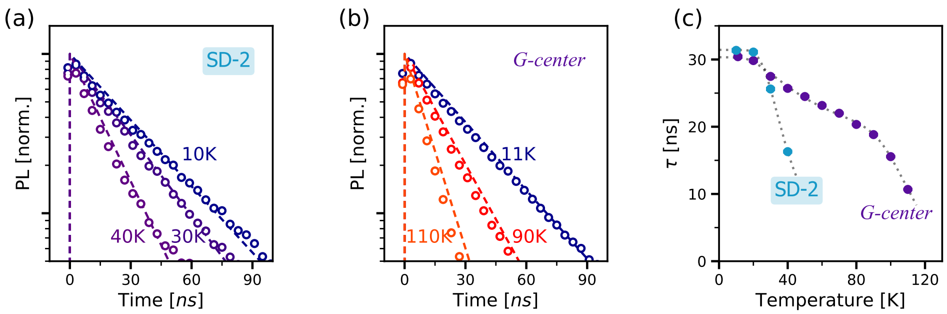


Figure. S-5. Time-resolved PL decay (in semi-log scale) of (a) a single G-center and (b) a single SD-2 center measured at different temperatures. The dashed lines represent data fitting with a single exponential function used to extract the excited state lifetime $\tau$. (c) Evolution of $\tau$ with temperature for the G-center and the SD-2 emitter. The dotted line is given as guide for the eye.

* anais.dreau@umontpellier.fr

[1] A. Beveratos, R. Brouri, J.-P. Poizat, and P. Grangier, “Bunching and Antibunching from Single NV Color Centers in Diamond,” in *Quantum Communication, Computing, and Measurement 3* (P. Tombesi and O. Hirota, eds.), pp. 261–267, Boston, MA: Springer US, 2002.

[2] K. P. O’Donnell, K. M. Lee, and G. D. Watkins, “Origin of the 0.97 eV luminescence in irradiated silicon,” *Physica B+C*, vol. 116, no. 1, pp. 258–263, 1983.

[3] G. Davies, “The optical properties of luminescence centres in silicon,” *Physics Reports*, vol. 176, pp. 83–188, May 1989.
